# Supplementary material for: Twisted Ways to Find Plane Structures in Simple Drawings of Complete Graphs
Source: arXiv:2203.06143 source file (2022-03-11)

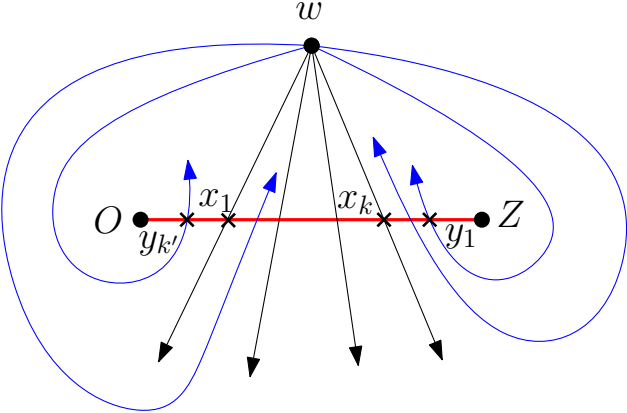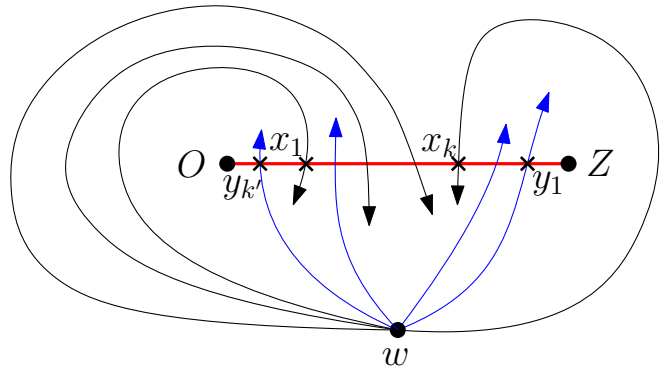

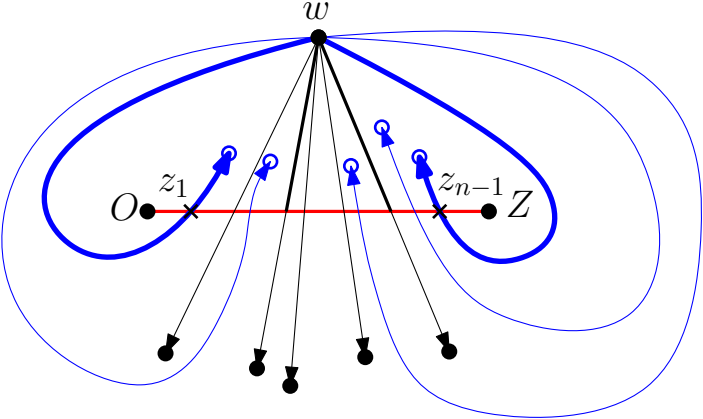

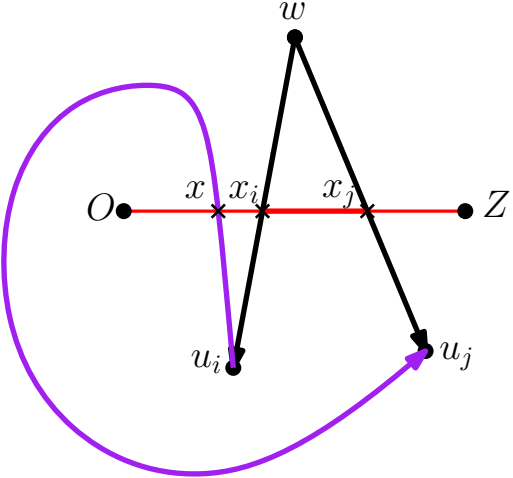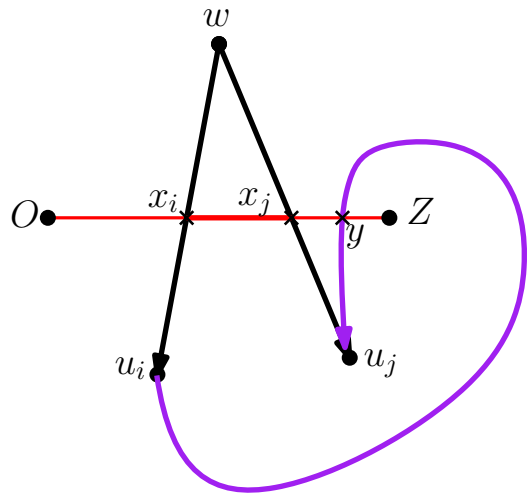

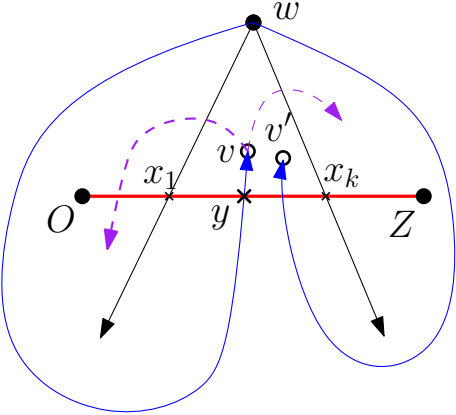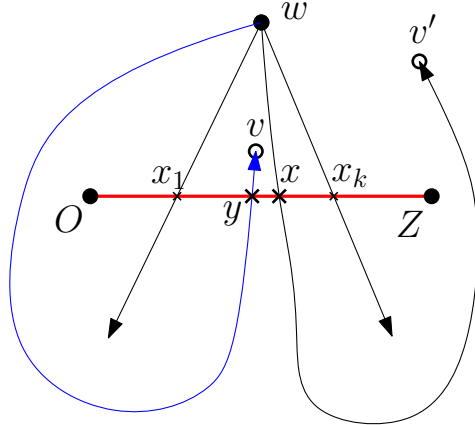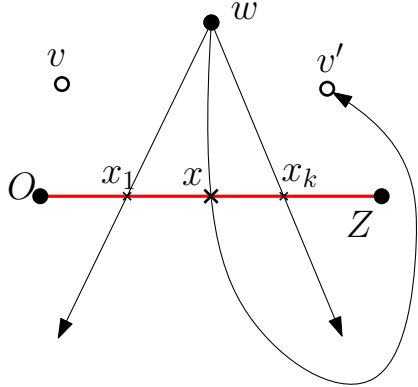

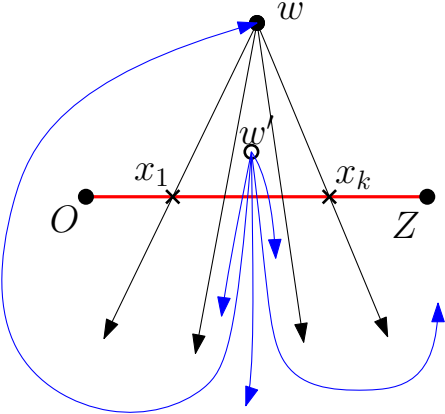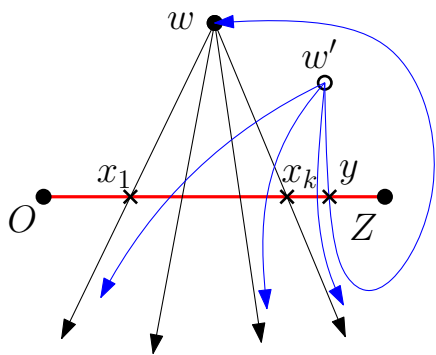

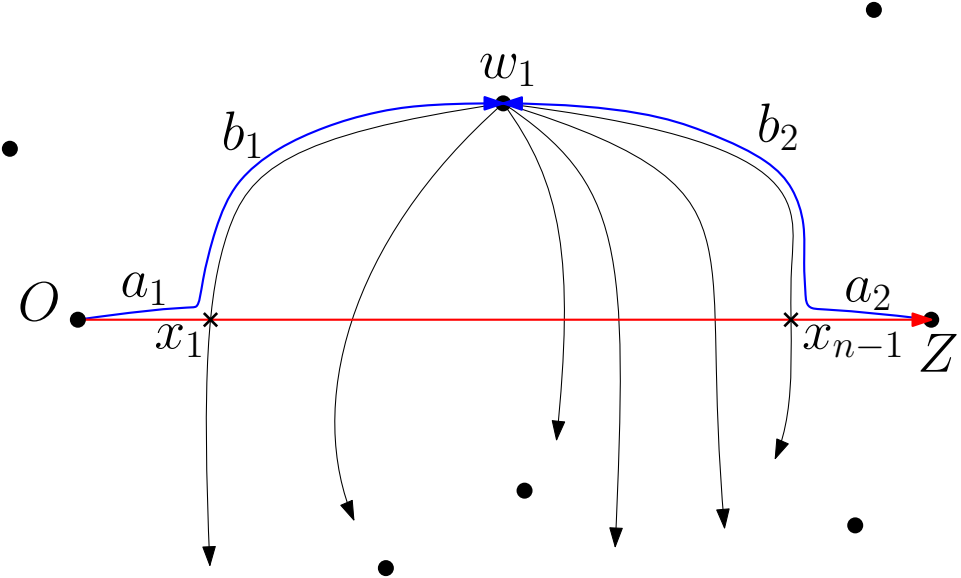

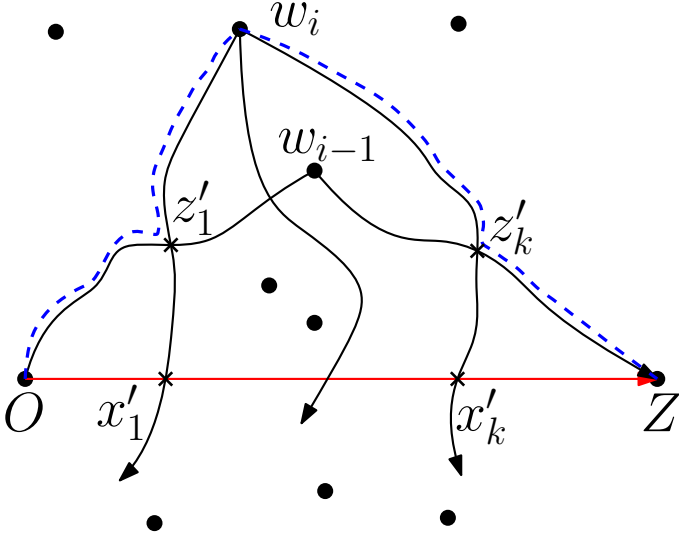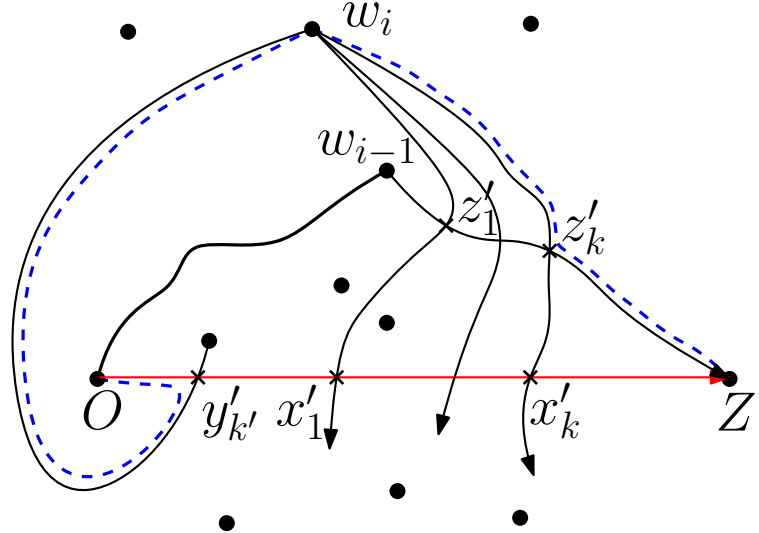

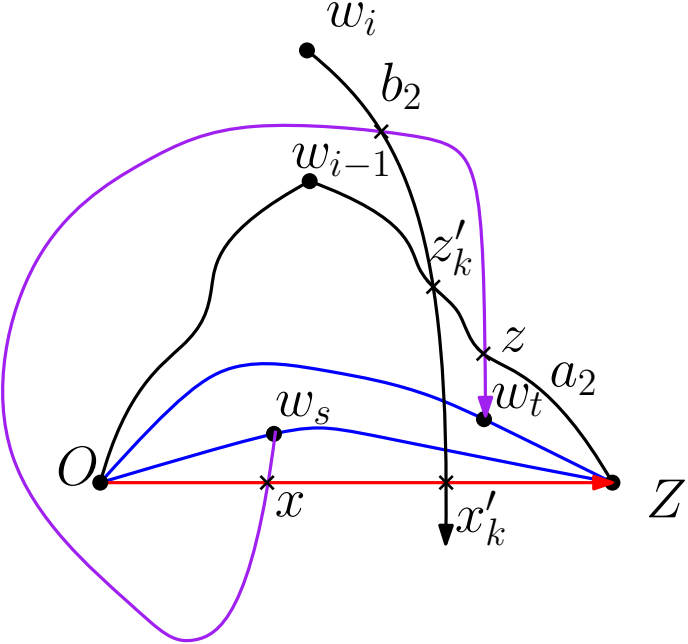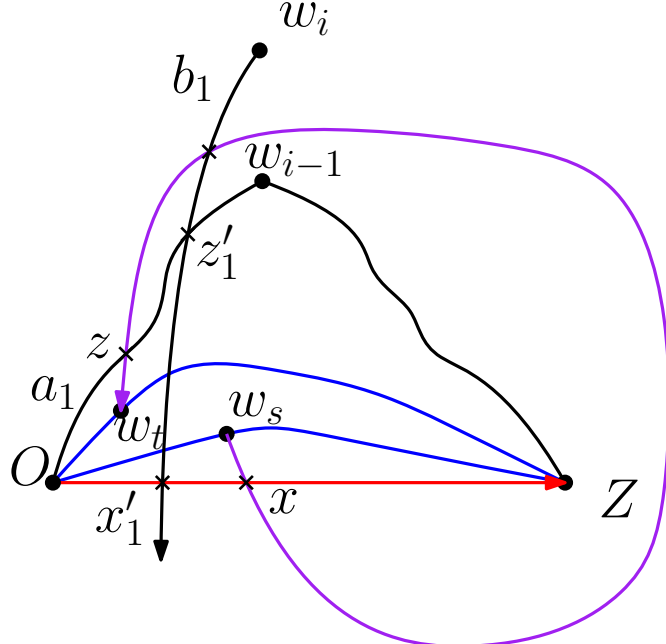



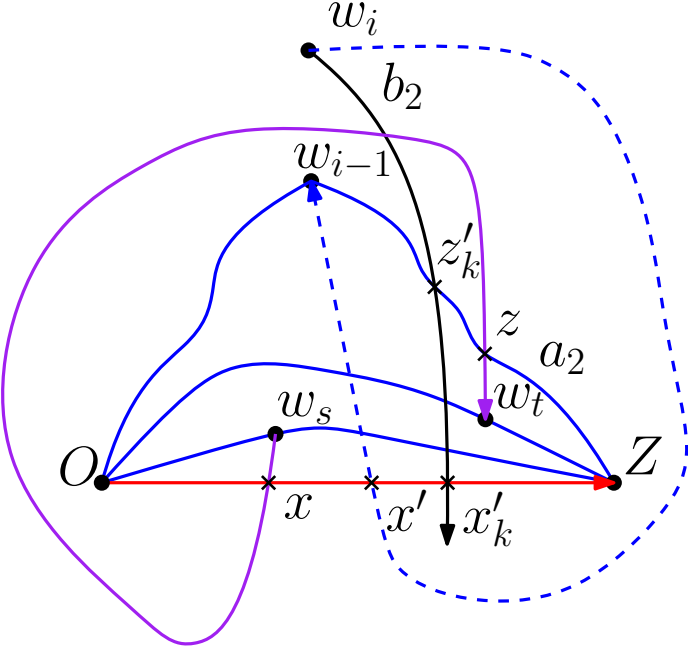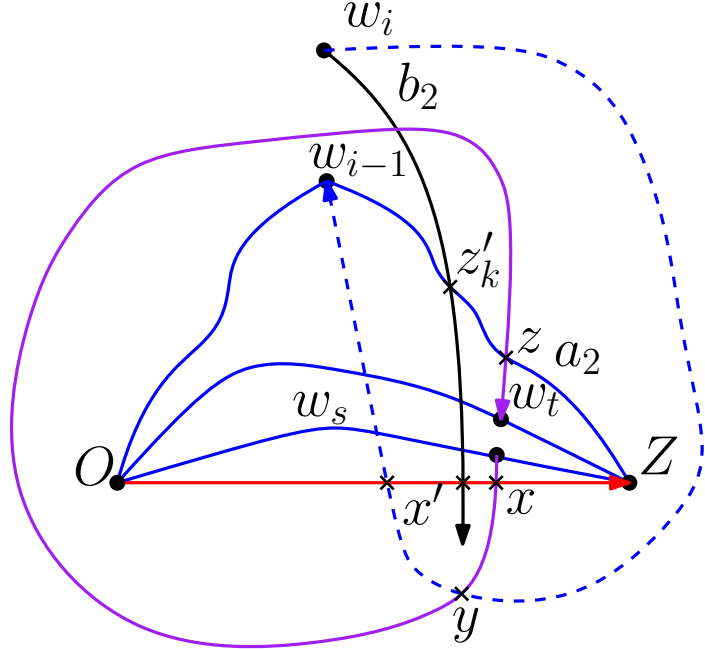

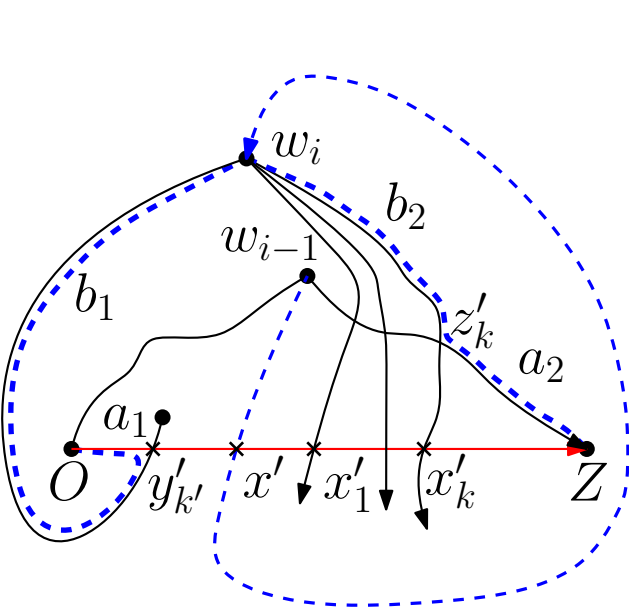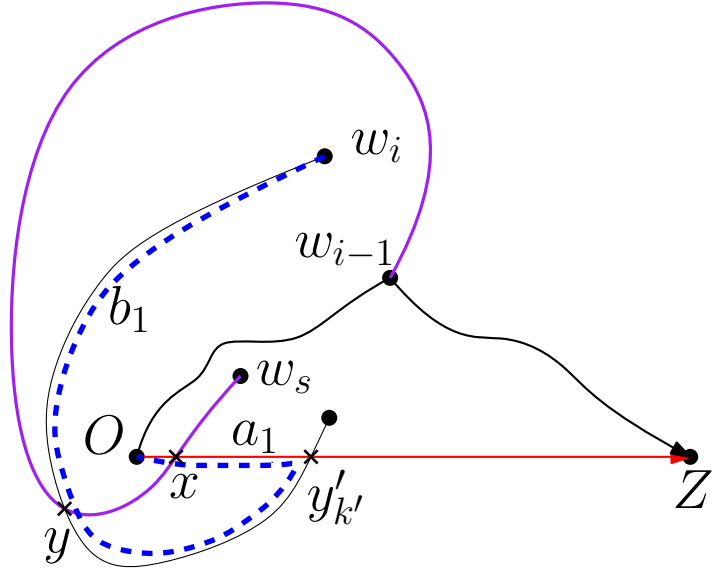

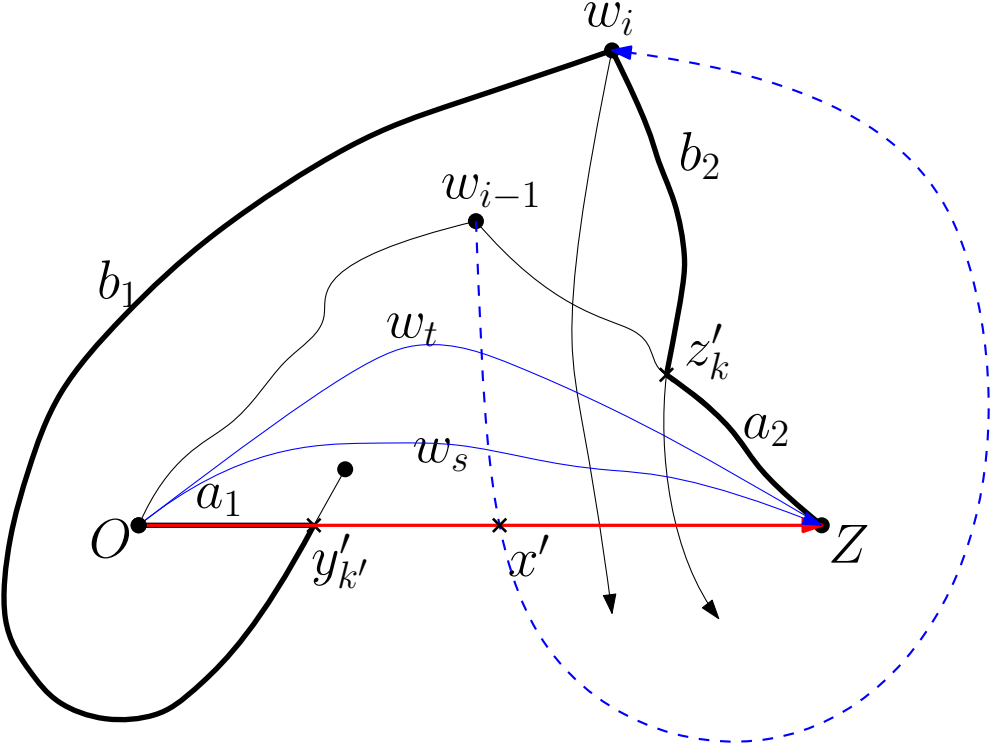

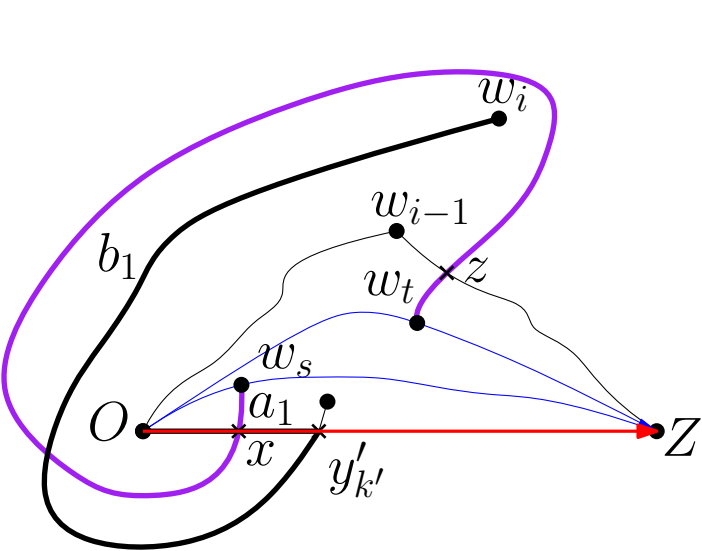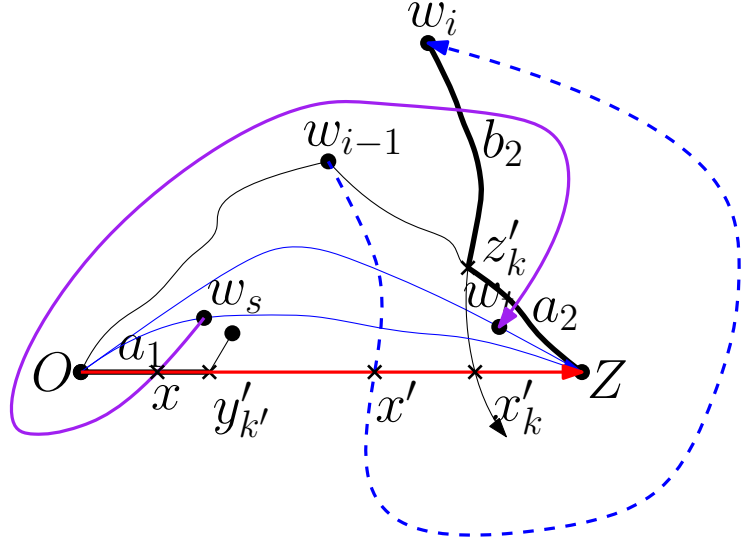

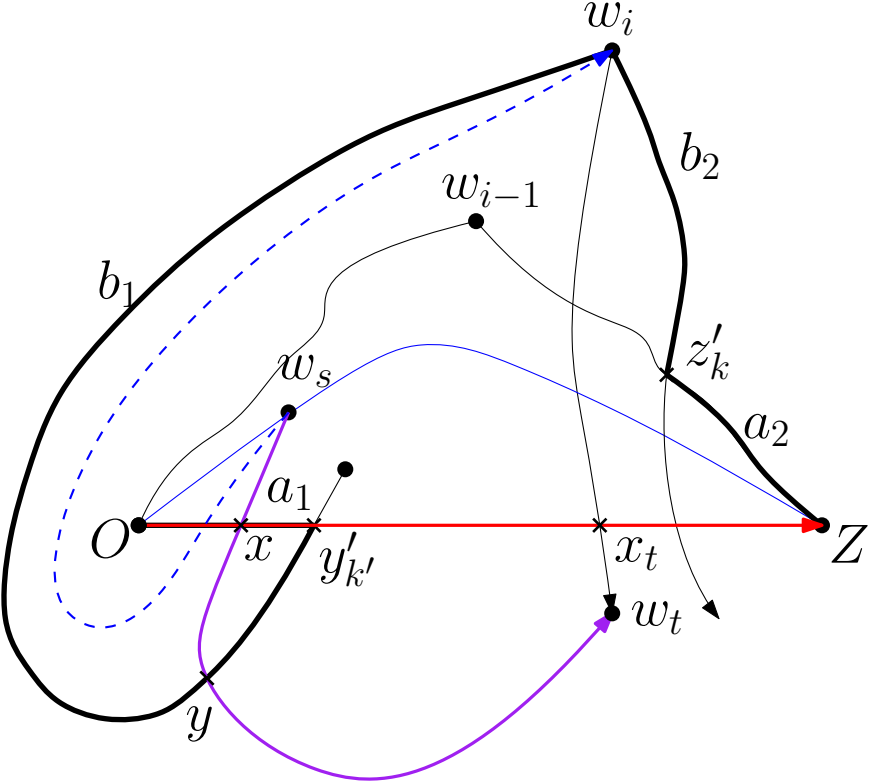

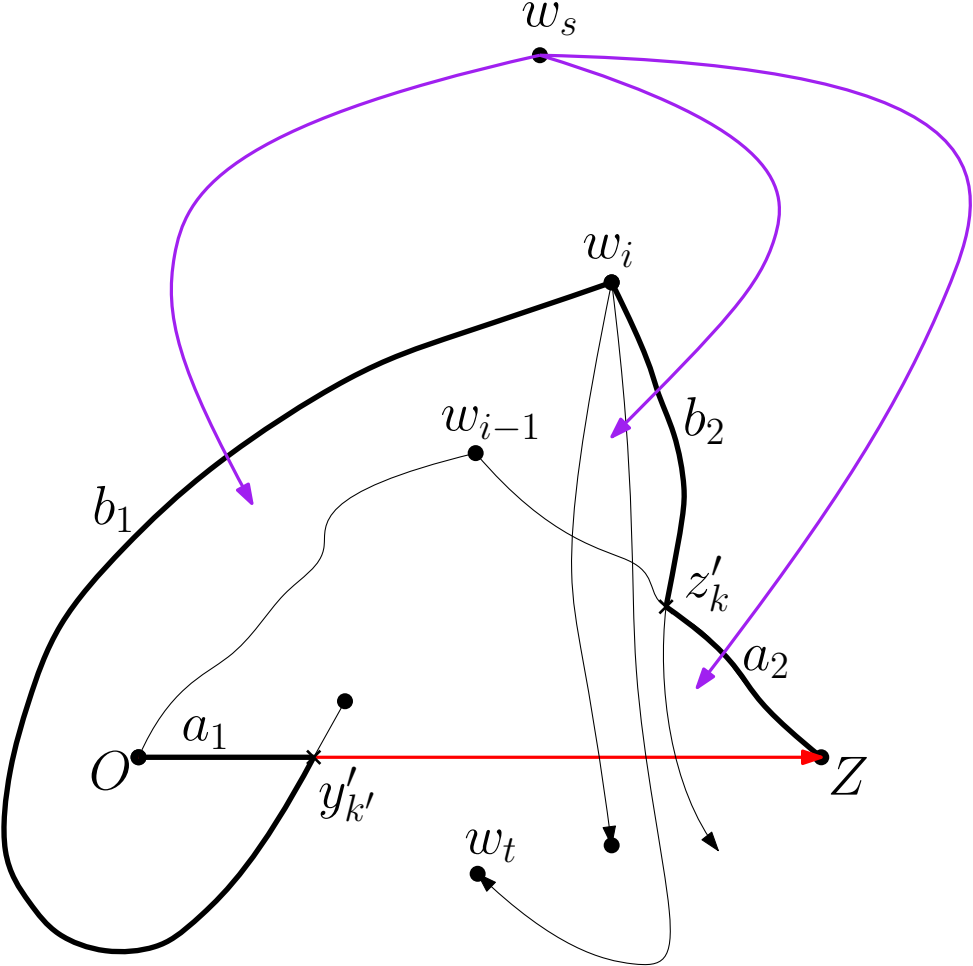

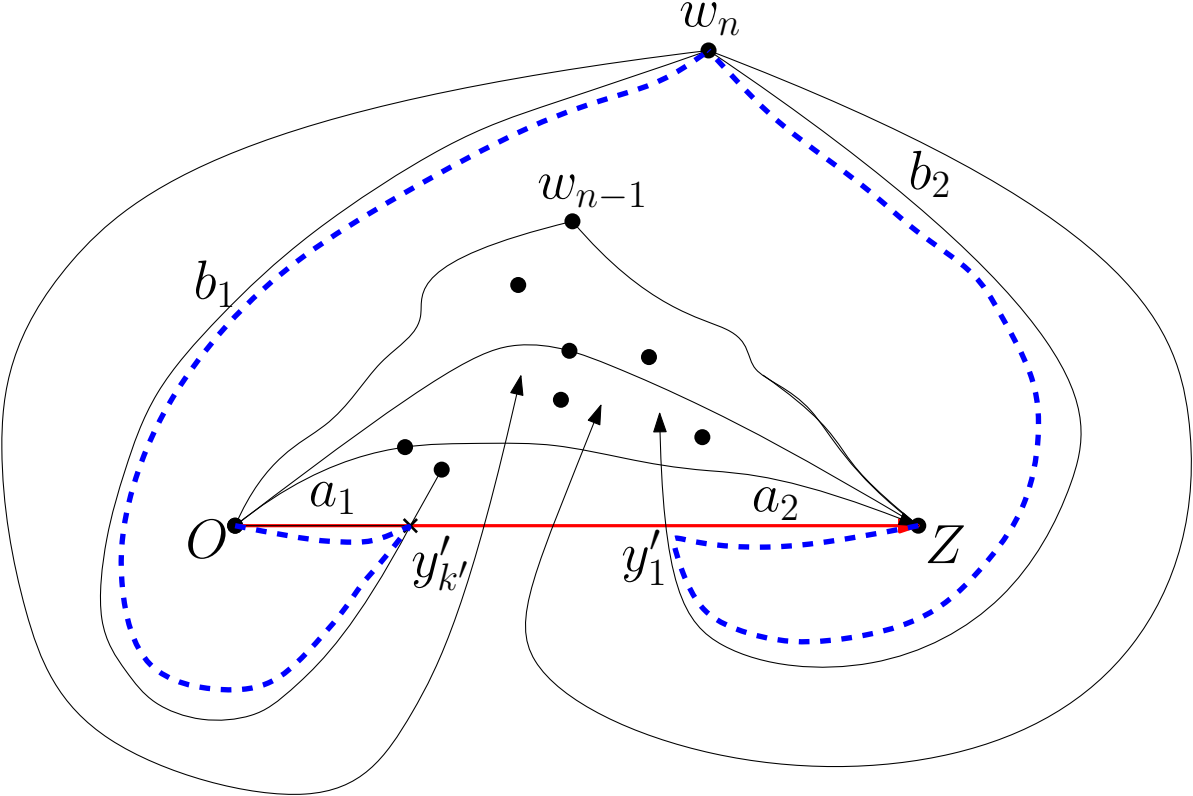

Supplement: Supplementary file 1 [file FigsAppendixC.pdf]
